# Supplementary material for: On the Transferability of Visual Features in Generalized Zero-Shot Learning
Source: arXiv:2211.12494 source file (2022-11-22)
Supplement: Supplementary file 1 [file 09.3_appendixC_additional_backbone_info_params_and_preDataset.tex]

% \section{Additional Feature Backbone Details}
% \label{sec:backbone_info}

% - Number of parameters
% - Dataset it was trained on
